# Supplementary material for: HoliSDiP: Image Super-Resolution via Holistic Semantics and Diffusion Prior
Source: arXiv:2411.18662 source file (2024-11-27)
Supplement: Supplementary file 1 [file design.tex]

\begin{figure}[t]
    \centering 
    \begin{subfigure}[b]{\linewidth}
        \centering
        \includegraphics[width=\linewidth]{Supplementary/figure/image/design/design-fusion.pdf}
    \end{subfigure}
    
    \centerline{\footnotesize (a) Input Fusion}
    \vspace{1mm}
    \begin{subfigure}[b]{\linewidth}
        \centering
        \includegraphics[width=\linewidth]{Supplementary/figure/image/design/design-t2i.pdf}
    \end{subfigure}
    \centerline{\footnotesize (b) T2I-Adapter}
    \caption{Alternative architectures for incorporating segmentation information. (a) Input Fusion primarily relies on the LR image for guidance, limiting semantic-aware detail generation. (b) T2I-Adapter combines guidance from separate adapters but fails to achieve enhancements in Real-ISR scenarios.}
    \label{fig:supp_design}
\end{figure}
